# Supplementary material for: Adaptive Space-Time Beamforming in Radar Systems
Source: arXiv:1302.2343 source file (2013-02-10)
Supplement: Supplementary file 1 [file appendix.tex]

\begin{appendix}
\chapter{Appendix}

\section{Appendices}\index{appendix}
Appendices should be used only when absolutely necessary. They
should come before the References. Sectional units are obtained
in the usual way, i.e. with the \LaTeX{} instructions
\verb|\section|, \verb|\subsection|.

If there is more than one appendix, number them alphabetically.
Number displayed equations occurring in the Appendix in this way,
e.g.~(\ref{appeq1}), (A.2), etc.

\begin{equation}
\mu(n, t) = \frac{\sum^\infty_{i=1} 1(d_i < t, N(d_i) = n)}
{\int^t_{\sigma=0} 1(N(\sigma) = n)d\sigma}\,. \label{appeq1}
\end{equation}

\begin{table}[h]
\tbl{Class options.$^{\textrm a}$}{
\begin{tabular}{@{}lll@{}}
\toprule
& \multicolumn{2}{c}{Purpose}\\[1pt]\cline{2-3}
\\[-6pt]
Option & Even page headers& Odd page headers\\\colrule
{\tt acrhead}& Author Name(s) & Chapter Title\\
{\tt csrhead}& Chapter Title & Section Title\\[6pt]
\begin{minipage}{.6in}{{\tt onethmnum}}\vspace*{51pt}\ \end{minipage} & \multicolumn{2}{l}{\begin{minipage}{2.3in}{To number all theorem-like objects in a
single sequence, e.g. Theorem~1, Definition 2,\\ Lemma 3, etc.\\
Default: individual numbering on different\\ theorem-like objects, e.g. Theorem 1,\\ Definition 1, Lemma 1, etc.}
\end{minipage}}\\
\\[-3pt]
{\tt draft} & \multicolumn{2}{l}{To draw border line around text area.}\\
& \multicolumn{2}{l}{Default: no border line around text area.}\\
\botrule
\end{tabular}}
\begin{tabnote}
$^{\textrm a}$Usage: \verb|\documentclass[option]{ws-book9x6}|
\end{tabnote}
\end{table}

\begin{table}[ht]
\tbl{Commonly used macros.}{
\begin{tabular}{@{}ll@{}}
\toprule
Macro/Environment name&Purpose\\
\colrule
{\tt$\backslash$chapter[\#1]}\{{\tt\#2}\} & Chapter title\\
{\tt$\backslash$section}\{{\tt\#1}\} & Section heading\\
{\tt$\backslash$subsection}\{{\tt\#1}\} & Subsection heading\\
{\tt$\backslash$subsubsection}\{{\tt\#1}\} & Subsubsection heading\\
{\tt$\backslash$section*}\{{\tt\#1}\} & Unnumbered Section head\\
{\tt$\backslash$begin}\{{\tt{itemlist}}\} & Start bulleted lists\\
{\tt$\backslash$end}\{{\tt{itemlist}}\} & End bulleted lists\\
{\tt$\backslash$begin}\{{\tt{arabiclist}}\} & Start arabic lists (1, 2, 3...)\\
{\tt$\backslash$end}\{{\tt{arabiclist}}\} & End arabic lists\\
{\tt$\backslash$begin}\{{\tt{romanlist}}\} & Start roman lists (i, ii, iii...)\\
{\tt$\backslash$end}\{{\tt{romanlist}}\} & End roman lists\\
{\tt$\backslash$begin}\{{\tt{Romanlist}}\} & Start roman lists (I, II, III...)\\
{\tt$\backslash$end}\{{\tt{Romanlist}}\} & End roman lists\\
{\tt$\backslash$begin}\{{\tt{alphlist}}\} & Start alpha lists (a, b, c...)\\
{\tt$\backslash$end}\{{\tt{alphlist}}\} & End alpha lists\\
{\tt$\backslash$begin}\{{\tt{Alphlist}}\} & Start alpha lists (A, B, C...)\\
{\tt$\backslash$end}\{{\tt{Alphlist}}\} & End alpha lists\\
{\tt$\backslash$begin}\{{\tt{proof}}\} & Start of Proof\\
{\tt$\backslash$end}\{{\tt{proof}}\} & End of Proof\\
{\tt$\backslash$begin}\{{\tt{theorem}}\} & Start of Theorem\\
{\tt$\backslash$end}\{{\tt{theorem}}\} & End of Theorem (see Page \pageref{theo} for detailed list)\\
{\tt$\backslash$begin}\{{\tt{appendix}}\} & Start Appendix\\
{\tt$\backslash$end}\{{\tt{appendix}}\} & End Appendix\\
{\tt$\backslash$begin}\{{\tt{thebibliography}}\}\{{\tt\#1}\} & Start of reference list\\
{\tt$\backslash$end}\{{\tt{thebibliography}}\} & End of reference list\\
{\tt$\backslash$bibitem}[\{{\tt\#1}\}]\{{\tt\#2}\}& reference item in author-date style\\
{\tt$\backslash$bibitem}\{{\tt\#1}\} & reference item in numbered style\\
{\tt$\backslash$bibliographystyle}\{{\tt\#1}\} & To include \btex{} style file\\
{\tt$\backslash$bibliography}\{{\tt\#1}\} & To include \btex{} database\\[6pt]
\multicolumn{2}{@{}l}{Macros available for Tables/Figures.}\\[3pt]
{\tt figure} & figures\\
{\tt sidewaysfigure} & landscape figures\\
{\tt table} & tables\\
{\tt sidewaystable} & landscape tables\\
{\tt$\backslash$tbl}\{{\tt\#1}\}\{{\tt\#2}\} & \#1 - table caption;\\
& \#2 - tabular environment\\[3pt]
\multicolumn{2}{@{}l}{Horizantal Rules for tables}\\
{\tt$\backslash$toprule} & one rule at the top\\
{\tt$\backslash$colrule} & one rule separating column heads from\\ & data cells\\
{\tt$\backslash$botrule} & one bottom rule\\
{\tt$\backslash$Hline} & one thick rule at the top and bottom of\\ & the tables with multiple column heads\\
\botrule
\end{tabular}}
\end{table}
\end{appendix}
